# Supplementary material for: Information flows in nanomachines
Source: arXiv:2312.02068 source file (2023-12-04)
Supplement: Supplementary file 1 [file appendix.tex]

%\documentclass[a4paper, onecolumn]{article}

%\usepackage[a4paper, total={7in, 9in}]{geometry}
%\usepackage{graphicx}
%\usepackage{hyperref}
%\usepackage{amsmath}
%\usepackage{xcolor}
%\usepackage{multicol}
%\usepackage{widetext}

%\begin{document}

\section{Thermodynamics and information flows in noisy systems}

In this appendix, we will prove the result $\eqref{eq:inform_flow_introduction}$ in a general case. To do this, consider a bipartite system composed of the subsystems $X, Y$, each one in contact with its respective thermal environment $E_X, E_Y$. Let $\rho(x,y)$ represent the probability density function of the global system, evolving following the Markovian master equation
\begin{equation}
    \frac{\partial\rho}{\partial t} = \mathcal{L}_X[\rho] + \mathcal{L}_Y[\rho].
    \label{eq:appendix_master}
\end{equation}
Here, $\mathcal{L}_{X,Y}[\rho]$ represents the evolution of the global system due to the action of the environment $E_{X,Y}$. For continuous bipartite systems, this equation is the Fokker-Planck equation,
\begin{equation}
    \mathcal{L}_X[\rho] = \frac{\partial[f(x)\rho]}{\partial x} + D_X \frac{\partial^2\rho}{\partial^2 x},
    \label{eq:general_fokker_planck}
\end{equation}
with $f(x)$ is a function of $x$ and $D_X$ a diffusion coefficient. For discrete systems, $\mathcal{L}_{X,Y}[\rho]$ are linear operators
\begin{equation}
    \left(\mathcal{L}_{X,Y}[\rho]\right)_i = \sum_j \Gamma_{ij}^{X,Y}\rho_j,
\end{equation}
with transition rates $\Gamma_{ij}^{X,Y}$. The marginal distributions of each subsystem were defined as
\begin{equation}
    \rho_X(x) = \int dy \rho(x,y),
\end{equation}
with analogous definitions for the subsystem $Y$ and discrete systems. Using Eq.\eqref{eq:appendix_master} one obtains
\begin{equation}
    \dot\rho_X = \mathcal{L}_X[\rho_X].
\label{eq:appendix_marginal_evo}
\end{equation}
Note that the last result requires independent baths, this is
\begin{equation}
     \int dy \mathcal{L}_Y[\rho] = 0.
\end{equation}

If the system evolves autonomously following Eq.\eqref{eq:appendix_master}, and $E_X$ and $E_Y$ have different temperature, the system reaches a NESS, where the system continuously exchanges energy and particles. Importantly, if the system is in contact with a single environment, for example $E_X$, it will reach an equilibrium state at temperature $T_X$ given by
\begin{equation}
    \mathcal{L}_X[\rho_\mathrm{eq}^X] = 0.
\end{equation}
The explicit form of the equilibrium state is given by the Gibbs ensemble
\begin{equation}
    \rho_\mathrm{eq}^X = \frac{1}{\mathcal{Z}_X}e^{-H(x,y)/kT_X},
\end{equation}
where $H(x,y)$ is the Hamiltonian acting on the joint system $X,Y$ and $\mathcal{Z}_X$ the partition function.

The heat $\dot Q_X$ was defined in the main text as the energy exchanged between the system and the environment $E_X$, this is
\begin{equation}
    \dot Q_X = \int dx dy H(x,y) \mathcal{L}_X[\rho\mathrm].
\end{equation}
The definition of $\dot Q_Y$ is analogous. Although I am considering a continuous system, this derivation is valid for discrete systems. Notice the following identity relating the heat with the steady state $\rho_\mathrm{eq}^X$,
\begin{equation}
    \log \rho_\mathrm{eq}^X + \log\mathcal{Z}_X = - H/kT_X,
\end{equation}
therefore
\begin{equation}
    -\frac{\dot Q_X}{kT_X} = \int dx dy \log \rho_\mathrm{eq}^X(x,y) \mathcal{L}_X[\rho\mathrm].
\end{equation}
\\

The local entropy production of the subsystem $X$ is
\begin{equation}
    S[\rho_X] = -\int dx dy \rho(x,y) \log \rho_X(x),
\end{equation}
and evolves following
\begin{equation}
\begin{split}
    \dot S_X &= -\int dx dy \left(\mathcal{L}_X[\rho] +\mathcal{L}_Y[\rho]  \right)\log \rho_X(x)
    \\&= -\int dx dy \mathcal{L}_X[\rho] \log \rho_X(x).
\end{split}
\end{equation}

To conclude, one must observe that
\begin{equation}
    -\int dx dy \mathcal{L}_X[\rho]\log \left(\frac{\rho}{\rho_\mathrm{eq}^X}\right) \geq 0.
\end{equation}
To see the positivity of this, consider Markovian evolution, then if $\rho > \rho_\mathrm{eq}^X$ the evolution holds $\mathcal{L}_X[\rho] < 0$ to drive $\rho$ towards $\rho_\mathrm{eq}^X$. In the opposite case, $\rho < \rho_\mathrm{eq}^X$ and the evolution holds $\mathcal{L}_X[\rho] > 0$; in both cases, the integrand is negative for any point, and the complete expression is positive.

The last observation consists in identify
\begin{equation}
    -\int dx dy \mathcal{L}_X[\rho]\log \left(\frac{\rho}{\rho_\mathrm{eq}^X}\right) =  \dot S_X - \dot Q_X /kT_X - \dot I_X  \geq 0,
\end{equation}
with
\begin{equation}
    \dot I_X = \int dx dy \mathcal{L}_X[\rho] \log\left(    \frac{\rho}{\rho_X}\right).
\end{equation}

%\end{document}
